# Supplementary material for: On the inverse cascade and flow speed scaling behavior in rapidly rotating Rayleigh-B\'enard convection
Source: arXiv:2003.01669 ancillary file (2020-03-03)
Supplement: Supplementary file 1 [file cascade-manuscript_supplementary_material.pdf]

# On the inverse cascade and flow speed scaling behavior in rapidly rotating Rayleigh-Bénard convection: Supplementary Material

**S. Maffei[1,3]†, M. J. Krouss[1], K. Julien[2] and M. A. Calkins[1]**

[1]Department of Physics, University of Colorado, Boulder, USA

[2]Department of Applied Mathematics, University of Colorado, Boulder, USA

[3]School of Earth and Environment, University of Leeds, Leeds, UK

(Received xx; revised xx; accepted xx)

† Email address for correspondence: S.Maffei@leeds.ac.uk

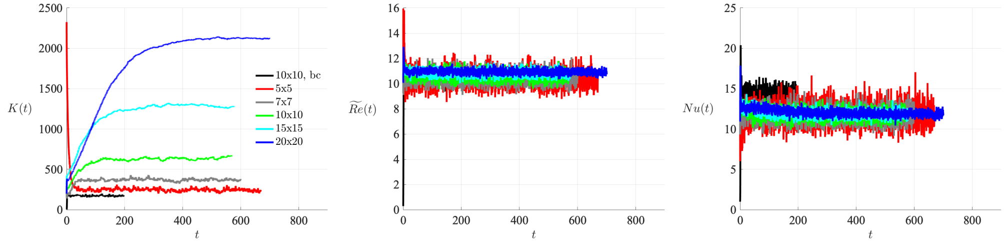


(a) $\widetilde{Ra} = 40, Pr = 1$ (b) $\widetilde{Ra} = 40, Pr = 1$ (c) $\widetilde{Ra} = 40, Pr = 1$

Figure 1: Time-series of simulations ($\widetilde{Ra} = 40, Pr = 1$) and different horizontal domain size in terms measured in amounts of critical wavelengths. The black curve represents a calculation with horizontal size $10\lambda_c \times 10\lambda_c$ where the variable $\langle\psi\rangle$ has been set to zero at the beginning of every timestep.

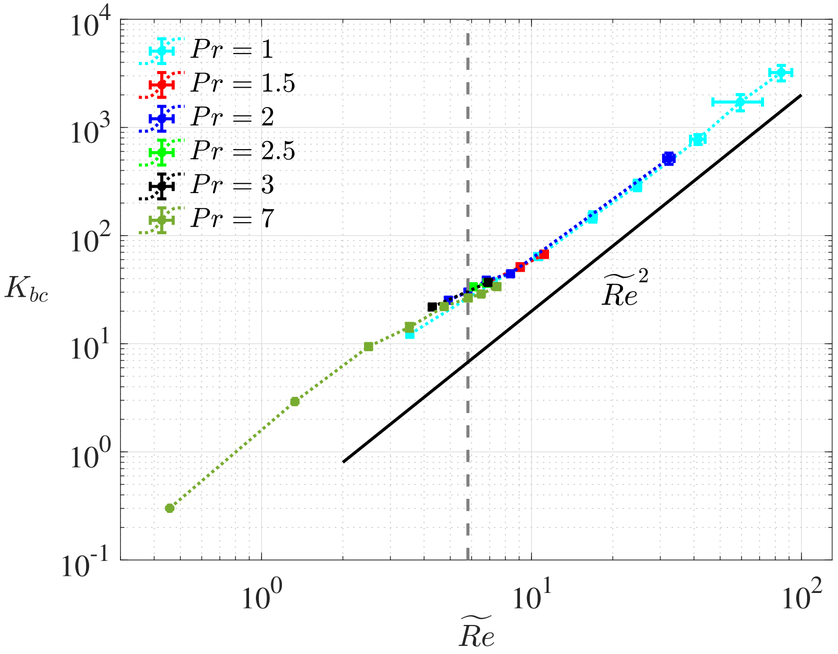


Figure 2: Time-averaged baroclinic kinetic energy, $K_{bc}$, as a function of the time-averaged Reynolds number $\widetilde{Re}$ and $Pr$. The black line, indicating the $\widetilde{Re}^2$ behavior is added for reference.
